# Supplementary material for: Speech-based Person Retrieval
Source: arXiv:2611.35952 source file (2026-11-26)
Supplement: Supplementary file 1 [file supp.tex]

\documentclass[10pt,twocolumn,letterpaper]{article}
\usepackage[review]{cvpr}
\usepackage{pifont}
\usepackage{subcaption}
\usepackage{amssymb}
\usepackage{multirow}
\usepackage[table]{xcolor}
\usepackage{makecell}
\usepackage{tcolorbox}
\usepackage{tabularx}
\definecolor{headgray}{gray}{0.9}

\usepackage{arydshln}
\setlength\dashlinedash{2pt}
\setlength\dashlinegap{1.5pt}

\makeatletter
\newcommand{\thickhline}{%
    \noalign {\ifnum 0=`}\fi \hrule height 0.7pt
    \futurelet \reserved@a \@xhline
}
\makeatother

\input{preamble}

\usepackage{xr-hyper}                 % 必须在 hyperref 之前
\definecolor{cvprblue}{rgb}{0.21,0.49,0.74}
\usepackage[pagebackref,breaklinks,colorlinks,allcolors=cvprblue]{hyperref}
\externaldocument[][nocite]{main}     % 读 main.aux 的公式/章节编号，不导入引用编号

\def\confName{CVPR}
\def\confYear{2027}
\title{Speech-based Person Retrieval}

\begin{document}
\input{sec/X_suppl}

% \clearpage
\clearpage
\global\vsize=\textheight

\raggedbottom
{
    \small
    \bibliographystyle{ieeenat_fullname}
    \bibliography{main}
}
\end{document}
